# Supplementary material for: Always on Voting: A Framework for Repetitive Voting on the Blockchain
Source: arXiv:2107.10571 source file (2023-09-24)
Supplement: Supplementary file 1 [file appendix03.tex]

Without AoV, an incumbent candidate  would  be voted again only during the next main election.
However, with AoV the elections are repeated at random time intervals between two main elections.
The incumbent candidate  may deviate from the median voters' ideal (in pursuit of reforms) but must not permit another candidate to cross the winning supermajority threshold, if they are to remain a winner.
One strategy to increase incumbent support while pursuing reforms is to reduce the costs to a fraction of the voters that are closer to the candidates' ideal with increased public spending.
Since public spending budgets are finite, it is possible for the incumbent to express public spending costs as a min-max optimization problem subject to the following constraints:
\begin{compactenum}
	\item[\textit{i.})] $t_1\leq spendingtime \leq t_2$,
	\item [\textit{ii.})] the area encompassing voters w.r.t. incumbent candidate voting ideal $>$ 1 - supermajority threshold.
\end{compactenum}

Due to the randomized nature of tally times with AoV, such optimal strategies found may be  diluted over  longer intervals of time.
It may occur that the incumbent was spending in one of the AoV intervals but he was not voted out.
However, if the spending stops, the costs to voters begin to accumulate and result in the incumbent candidate losing in a future interval.
It implies that the incumbent will have to continue spending in the next interval.
Another incumbent strategy (constraint \textit{i.}) would be to distribute public spending across all intervals where reforms are pursued.
However, only a fraction of the finite public spending budget may be used in each interval, and their effects are diluted across the AoV intervals.
